# Supplementary material for: A challenge to the Delta G~0 interpretation of hydrogen evolution
Source: arXiv:1903.09903 ancillary file (2019-10-04)
Supplement: Supplementary file 1 [file SupportingInformation.pdf]

**Supporting information:**

# A challenge to the $\Delta G{\sim}0$ interpretation of hydrogen evolution

Per Lindgren, Georg Kastlunger, and Andrew A. Peterson*

*School of Engineering, Brown University, Providence, Rhode Island, 02912, USA*

E-mail: andrew_peterson@brown.edu

## Contents

**1 A Decoupled Computational Electrode Model** **3**
1.1 Potential-controlled computational electrode . . . 3
1.2 Thermodynamically-consistent reaction barriers . . . 4
1.3 Unified treatment of "non"-electrochemical steps . . . 5

**2 Free energy diagrams for competing pathways** **6**

**3 Tabulated free energy reaction energies and barriers** **6**

**4 Minimum energy pathway of Tafel starting from two fcc hollow sites** **11**

**5 Minimum energy pathway of Volmer reaction into fcc site** **11**

**6 Elementary step electron transfer** **11**

**7 Microkinetic model** **15**
7.1 Volmer–Heyrovsky mechanism . . . 15
7.2 Top-hollow Volmer–Tafel . . . 17
7.3 Top-top Volmer–Tafel . . . 18
7.4 Potential dependence . . . 18

**8 Interpretation of Tafel slopes** **18**
8.1 Volmer . . . 20
8.2 Heyrovsky . . . 22
8.3 Top-top Tafel . . . 23
8.4 Top-hollow Tafel . . . 24

**9 Linear response between reaction energy and applied potential** **27**

**10 Volmer reaction energetics as a function of unit cell size** **27**

**11 Tafel reaction energetics as a function of water geometry** **28**

**12 Potential energy barriers on Au(111)** **29**

**13 Volmer reaction on Au(111) with different water geometries** **29**

**14 Site-dependent Tafel reaction barriers** **30**

**15 Tafel barrier rationalization on the basis of a normal mode analysis** **30**

**16 Unit cell in SJ method** **31**

**References** **34**

# 1 A Decoupled Computational Electrode Model

The computational hydrogen electrode (CHE) approach[1] has been tremendously successful in facilitating the simulation of electrochemical reactions. Part of the allure of the CHE method is that the chemical potential of the proton/electron pair can be abstracted, and replaced with the simpler-to-calculate chemical potential of $H_2$. However, in a reaction barrier calculation the proton is intimately involved, and the number of electrons changes continuously to hold the potential constant. Here, we describe how this can be treated in a thermodynamic manner consistent with the (potential-controlled) CHE method. This assures thermodynamic consistency in the treatment of reaction kinetics.

## 1.1 Potential-controlled computational electrode

Say that we would like to understand an elementary reaction, that takes place at a specified electrode potential $\phi$:

$$* + \mathrm{H}^+ + (1+\epsilon)\mathrm{e}^- \longrightarrow \mathrm{H}* \tag{1}$$

where $*$ indicates the electrocatalyst surface. In the traditional CHE treatment $\epsilon$ is taken to be zero—that is, an integer electron is assumed to be transferred—however, we'll note that this isn't necessarily the case when the potential is kept constant, as the two different surface states ($*$ *vs.* H$*$) may require slightly different charging to maintain the potential, due to differences in surface dipoles. To be clear, we are not claiming that electrons are not quantized. In a physical system, the potentiostat keeps the potential constant by injecting electrons into an electrode that consists of a huge number of atoms and active sites—even a tiny 2-nm particle contains hundreds of atoms—and in practice the constant-potential condition can still be maintained via integer numbers of electrons. However, a consequence is that the number of electrons for an elementary step can still be a non-integer quantity at constant potential. However, for the overall half-reaction $2\mathrm{H}^+ + 2\mathrm{e}^- \longrightarrow \mathrm{H}_2$, there are undoubtedly two integer electrons involved, as in this catalytic cycle the surface state is unchanged.

The free energy change of this reaction, at the fixed potential $\phi$, is

$$\Delta G^{\phi}_{\mathrm{rxn}} = \mu^{\phi}[\mathrm{H}*] - \mu^{\phi}[*] - \mu^{\circ}[\mathrm{H}^+] - (1+\epsilon)\mu^{\phi}[\mathrm{e}^-]$$

where $\mu^{\phi}$ indicates the chemical potential at electrode potential $\phi$. The chemical potential of the proton is that in the bulk solution, which for simplicity we take at a pH value of 0 (as indicated by the $^\circ$ on the proton's chemical potential), but this could easily be adjusted thermodynamically with $\mu[\mathrm{H}^+] = \mu^{\circ}[\mathrm{H}^+] - \ln 10 \cdot k_{\mathrm{B}}T \cdot \mathrm{pH}$.

As in the CHE model, we recognize that 0 $\mathrm{V_{SHE}}$ (standard hydrogen electrode) is defined when the reaction $\frac{1}{2}\mathrm{H}_2 \longleftrightarrow \mathrm{H}^+ + \mathrm{e}^-$ is in equilibrium; thermodynamically, this means

$$\mu^{\circ}[\mathrm{H}^+] + \mu^{0\mathrm{V}}[\mathrm{e}^-] = \frac{1}{2}\mu^{\circ}[\mathrm{H}_2] \tag{2}$$

where $H_2$ is taken at standard pressure and the reaction temperature; in the SHE definition,

the protons are at pH 0. Substituting this into the prior equation allows us to write:

$$\Delta G^{\phi}_{\mathrm{rxn}} = \mu^{\phi}[\mathrm{H}*] - \mu^{\phi}[*] - \frac{1}{2}\mu^{\circ}[\mathrm{H}_2] + \underbrace{\left(\mu^{0\mathrm{V}}[\mathrm{e}^-] - \mu^{\phi}[\mathrm{e}^-]\right)}_{=e\phi} - \epsilon\mu^{\phi}[\mathrm{e}^-]$$

where we note that the difference in chemical potentials of an electron at 0 $\mathrm{V}_{\mathrm{SHE}}$ and $\phi$ is simply $e\phi$, if $\phi$ is expressed on the SHE scale. This simplifies to

$$\boxed{\Delta G^{\phi}_{\mathrm{rxn}} = \mu^{\phi}[\mathrm{H}*] - \mu^{\phi}[*] - \epsilon\mu^{\phi}[\mathrm{e}^-] - \frac{1}{2}\mu^{\circ}[\mathrm{H}_2] + e\phi} \quad (3)$$

We would refer to the above as a truly constant-potential computational electrode formulation, and it is used in the current work to find the energy changes between stable states in the reported free energy diagrams.

Constant-potential methodologies, such as the solvated jellium method, allow the direct control of the potential by varying the number of electrons in the system. Within this framework, $\mu^{\phi}[\mathrm{H}*]$ and $\mu^{\phi}[*]$ are calculated as the vibrational free energies of H* and * at the applied charge corresponding to $\phi$, respectively. In our implementation of the SJ method, the potential energy returned by the electronic structure calculator automatically adjusts the result by $n\mu^{\phi}[\mathrm{e}^-]$, where $n$ is the charge required to achieve the specified potential $\phi$ and $\mu^{\phi}[\mathrm{e}^-]$ is the Fermi energy, referenced to the field-free region in the (implicit) solvent close to the interface;[2,3] thus, the $\epsilon\mu^{\phi}[\mathrm{e}^-]$ term is included immediately.

The conventional CHE approach can be recovered by taking $\epsilon$ to be zero, while the chemical potentials would be taken in the canonical framework, where the potential (Fermi level) is not necessarily constant. This will lead to a slight deviation from truly constant-potential conditions. In our experience, this deviation is small, which has made the CHE model an excellent approach for the simulation of elementary reaction energies.

## 1.2 Thermodynamically-consistent reaction barriers

In the example reaction (1), the proton $\mathrm{H}^+$ can be thought of as existing in a thermodynamic reservoir. Before simulating the reaction barrier, the proton must be brought from the reservoir to near the electrode surface; this is shown schematically in Figure S1. Here, we describe how we incorporate both this proton-shuttling step and the surface reaction barriers in a thermodynamically consistent manner, again accounting for the partial charge transfer along the constant-potential reaction pathway. Note that the amount of charge transfer—which can be thought of as electrons injected by the potentiostat—is a continuous variable along the reaction path; this is shown later in Fig. S6.

Recently, Chen and co-workers[4] elegantly showed that solvated protons located near the electrode pre-hybridize with the electrode surface, resulting in a partial charge transfer. Our constant-potential simulations are in full agreement with this view, where we consistently observe a net charge transfer associated with this step, typically on the order of 0.2–0.5 electrons.

Let's say the reaction to an arbitrary point along the reaction path, such as the transition state, is

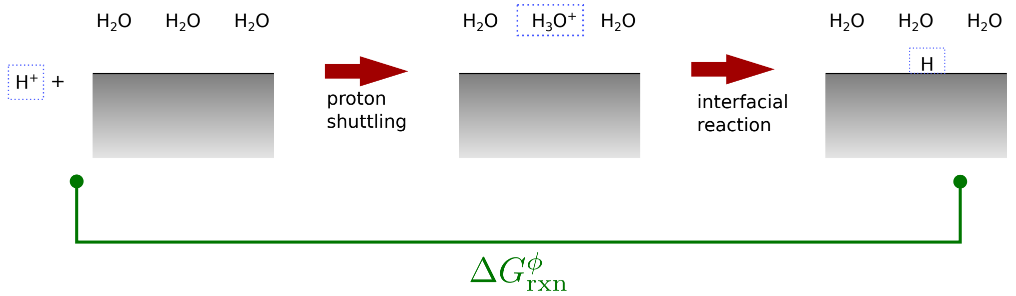


**Figure S1:** The proton must be brought from a thermodynamic reservoir before it can react.

$$* + H^+ + xe^- \longrightarrow H{-}*$$

where H−∗ indicates the reacting complex; that is, the hydrogen–surface bond that is forming. We can relate the free energy of this point along the path, $G^\phi_{\text{path}}$, to that of the initial state, $G^\phi_{\text{IS}}$, at constant potential $\phi$ as

$$G^\phi_{\text{path}} - G^\phi_{\text{IS}} = \mu^\phi[\text{H}{-}*] - \mu^\phi[*] - x\mu^\phi[\text{e}^-] - \mu^\circ[\text{H}^+]$$

where we again take the pH to be zero, but this could be adjusted as described above in footnote 1.1. As before, we use the CHE relation (eq. (2)) to substitute for $\mu^\circ[\text{H}^+]$:

$$G^\phi_{\text{path}} - G^\phi_{\text{IS}} = \mu^\phi[\text{H}{-}*] - \mu^\phi[*] - x\mu^\phi[\text{e}^-] - \frac{1}{2}\mu^\circ[\text{H}_2] + \mu^{0\text{V}}[\text{e}^-]$$

$$\boxed{G^\phi_{\text{path}} - G^\phi_{\text{IS}} = \mu^\phi[\text{H}{-}*] - \mu^\phi[*] + (1-x)\mu^\phi[\text{e}^-] - \frac{1}{2}\mu^\circ[\text{H}_2] + e\phi} \tag{4}$$

This equation can be used to find the free energy at any point along the reaction path, and is particularly useful for deriving the transition-state free energy of an electrochemical reaction. Note that it is functionally identical to eq.(3); this is important, as it means that the endstate energetic as calculated along the reaction path is consistent with the (potential-controlled) CHE.

## 1.3 Unified treatment of "non"-electrochemical steps

The approach we take above unifies a CHE-like model for the elementary step with that of the reaction barrier. Interestingly, the approach even generalizes to non-electrochemical reactions. For example, consider that the Tafel $H_2$-liberating reaction can be written as

$$2\text{H}* + xe^- \longrightarrow 2* + \text{H}_2$$

Conventionally, one wouldn't include any electrons in this reaction, and would refer to it as a non-electrochemical step. However, by identical logic as that used when discussing the Volmer step at constant potential, we argue that if the electrode potential is kept constant, then the possibility of electron transfer *must* be allowed for, as these are conjugate variables. (*I.e.*, in both physical potentiostats and our model, the electrode potential is kept constant

by varying the number of electrons in the system; this offsets changes in the workfunction induced by the presence of adsorbates on the surface.) Thus, we can expect $x$ will typically be a number close to but not identically 0, for the same reason that $(1+\epsilon)$ will be a number close to but not identically 1 in the Volmer step.

We can treat this step in an identical method as before, and express the free-energy change at constant potential $\phi$ as

$$\Delta G^{\phi}_{\mathrm{rxn}} = 2\mu^{\phi}[*] - 2\mu^{\phi}[\mathrm{H}*] - x\mu^{\phi}[\mathrm{e}^{-}] + \frac{1}{2}\mu[\mathrm{H}_2]$$

as before, the SJ calculator automatically adjusts the energies ($n\mu^{\phi}[\mathrm{e}^{-}]$), where $n$ is the charge required to achieve the potential $\phi$.

Thus, we treat electrochemical and non-electrochemical elementary steps *identically.* This is a departure from previous theoretical treatments: we do not decide in advance which steps are and are not electrochemical; we can instead assess this by examining $x$ after the constant-potential calculations. Thus, this can be considered a fully *unified* treatment: barriers are treated the same as endstates, and electrochemical steps are treated the same as non-electrochemical steps.

# 2 Free energy diagrams for competing pathways

Free energy diagrams for Volmer–Heyrovsky (via top hydrogen) and Volmer–Tafel (via top–hollow hydrogen) are shown in Figures S2 and S3.

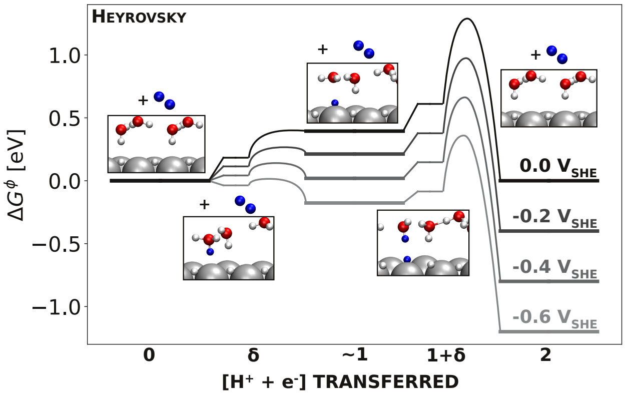


**Figure S2:** Free energy diagram for the Volmer–Heyrovsky mechanism at $U \leq 0$ $\mathrm{V_{SHE}}$.

# 3 Tabulated free energy reaction energies and barriers

The tables below contain numerical values for the free energy reaction energies and barriers of all elementary steps in Figures 3, S4 and S5. Here, we include two tables for each elementary electrochemical step: one for the fractional charge transfer energetics, and one where we include the shuttling of a bulk solvated proton into the electrochemical double layer. The

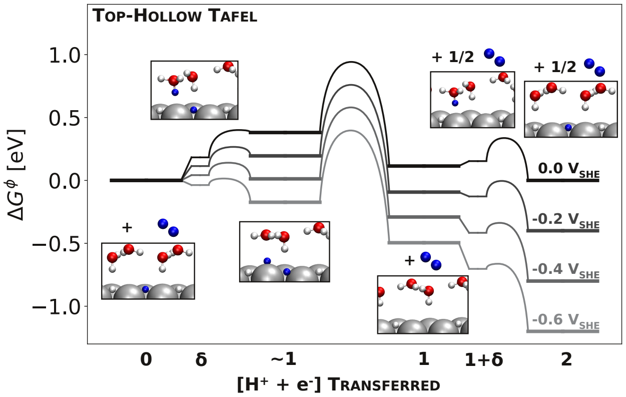


**Figure S3:** Free energy diagram for the top–hollow Volmer–Tafel mechanism at $U \leq 0$ $V_{SHE}$.

latter has an additional barrier coming from the energetic difference between the proton in the electrochemical interface and its bulk solvated counterpart. Note that we cannot calculate barriers for the proton shuttling; we simply calculate the relative stability of the states and add this difference to the calculated reaction barriers. These values represent the complete elementary steps (*i.e.*, integer electron transfer).

### Volmer $\Theta_{\rm H}$=1 $\rightarrow$ $\Theta_{\rm H}$= $\frac{7}{6}$; top adsorption

**Fractional charge transfer**

Average charge transfer, $\Delta\bar{n}$=0.525

| **Potential V vs. SHE** | $\Delta\Delta G^{\rm r}_{\Phi_{\rm e}}$ (eV) | $\Delta G^{\ddagger}_{\Phi_{\rm e}}$ (eV) | $\Delta n$ |
|---|---|---|---|
| 0.0 | 0.211 | 0.222 | 0.524 |
| -0.1 | 0.159 | 0.187 | 0.521 |
| -0.2 | 0.081 | 0.152 | 0.526 |
| -0.3 | 0.047 | 0.124 | 0.524 |
| -0.4 | -0.042 | 0.098 | 0.529 |
| -0.5 | -0.076 | 0.074 | 0.525 |
| -0.6 | -0.158 | 0.053 | 0.525 |

**Elementary-step charge transfer**

| **Potential V vs. SHE** | $\Delta G^{\rm r}_{\Phi_{\rm e}}$ (eV) | $\Delta G^{\ddagger}_{\Phi_{\rm e}}$ (eV) |
|---|---|---|
| 0.0 | 0.394 | 0.405 |
| -0.1 | 0.307 | 0.335 |
| -0.2 | 0.213 | 0.266 |
| -0.3 | 0.120 | 0.197 |
| -0.4 | 0.019 | 0.140 |
| -0.5 | -0.075 | 0.075 |
| -0.6 | -0.177 | 0.0150 |

## Volmer $\Theta_{\mathrm{H}}=\frac{5}{6} \rightarrow \Theta_{\mathrm{H}}=1$; fcc-hollow adsorption

### Fractional charge transfer

Average charge transfer, $\Delta\bar{n}=0.575$

| **Potential V vs. SHE** | $\Delta G^{\mathrm{r}}_{\Phi_{\mathrm{e}}}$ (eV) | $\Delta G^{\ddagger}_{\Phi_{\mathrm{e}}}$ (eV) | $\Delta n$ |
|---|---|---|---|
| 0.0 | -0.153 | 0.183 | 0.598 |
| -0.1 | -0.215 | 0.147 | 0.595 |
| -0.2 | -0.273 | 0.123 | 0.589 |
| -0.3 | -0.330 | 0.096 | 0.584 |
| -0.4 | -0.383 | 0.079 | 0.562 |
| -0.5 | -0.438 | 0.058 | 0.556 |
| -0.6 | -0.497 | 0.041 | 0.544 |

### Elementary-step charge transfer

| **Potential V vs. SHE** | $\Delta G^{\mathrm{r}}_{\Phi_{\mathrm{e}}}$ (eV) | $\Delta G^{\ddagger}_{\Phi_{\mathrm{e}}}$ (eV) |
|---|---|---|
| 0.0 | -0.164 | 0.173 |
| -0.1 | -0.256 | 0.106 |
| -0.2 | -0.357 | 0.039 |
| -0.3 | -0.453 | Activationless |
| -0.4 | -0.559 | Activationless |
| -0.5 | -0.661 | Activationless |
| -0.6 | -0.755 | Activationless |

**Heyrovsky $\Theta_H=\frac{7}{6} \rightarrow \Theta_H=1$; top adsorbed hydrogen + $(H^+ + e^-)$**

**Fractional charge transfer**

Average charge transfer, $\bar{n}$=0.685

| **Potential V vs. SHE** | $\Delta G^{r}_{\Phi_e}$ (eV) | $\Delta G^{\ddagger}_{\Phi_e}$ (eV) | $\Delta n$ |
|---|---|---|---|
| 0.0 | -0.611 | 0.678 | 0.698 |
| -0.1 | -0.694 | 0.639 | 0.694 |
| -0.2 | -0.777 | 0.597 | 0.690 |
| -0.3 | -0.860 | 0.553 | 0.686 |
| -0.4 | -0.947 | 0.516 | 0.679 |
| -0.5 | -1.03 | 0.481 | 0.675 |
| -0.6 | -1.11 | 0.445 | 0.671 |

**Elementary-step charge transfer**

| **Potential V vs. SHE** | $\Delta G^{r}_{\Phi_e}$ (eV) | $\Delta G^{\ddagger}_{\Phi_e}$ (eV) |
|---|---|---|
| 0.0 | -0.394 | 0.895 |
| -0.1 | -0.507 | 0.826 |
| -0.2 | -0.612 | 0.762 |
| -0.3 | -0.720 | 0.693 |
| -0.4 | -0.819 | 0.644 |
| -0.5 | -0.925 | 0.583 |
| -0.6 | -1.02 | 0.536 |

**Tafel $\Theta_H=\frac{7}{6} \rightarrow \Theta_H=\frac{5}{6}$; top + hollow**

| **Potential V vs. SHE** | $\Delta G^{r}_{\Phi_e}$ (eV) | $\Delta G^{\ddagger}_{\Phi_e}$ (eV) |
|---|---|---|
| 0.0 | -0.217 | 0.561 |
| -0.1 | -0.233 | 0.562 |
| -0.2 | -0.238 | 0.565 |
| -0.3 | -0.246 | 0.564 |
| -0.4 | -0.253 | 0.568 |
| -0.5 | -0.258 | 0.567 |
| -0.6 | -0.272 | 0.570 |

**Tafel $\Theta_{\mathrm{H}}=\frac{8}{6} \rightarrow \Theta_{\mathrm{H}}=1$; top + top**

| **Potential V vs. SHE** | $\Delta G^{\mathrm{r}}_{\Phi_\mathrm{e}}$ (eV) | $\Delta G^{\ddagger}_{\Phi_\mathrm{e}}$ (eV) |
|---|---|---|
| 0.0 | -0.859 | 0.286 |
| -0.1 | -0.874 | 0.285 |
| -0.2 | -0.884 | 0.285 |
| -0.3 | -0.895 | 0.286 |
| -0.4 | -0.914 | 0.286 |
| -0.5 | -0.919 | 0.292 |
| -0.6 | -0.934 | 0.296 |

# 4 Minimum energy pathway of Tafel starting from two fcc hollow sites

Figure S4 shows the minimum energy pathway of the Tafel reaction between two fcc-adsorbed hydrogen atoms at the equilibrium potential. As shown in the main article, we typically simulate this elementary reaction by combining an $H_{top}$ (top adsorbed) species with an $H_{fcc}$ (fcc-hollow adsorbed) or another $H_{top}$ species. However, the combination of two $H_{fcc}$ species is not included. The reason for this is shown in Figure S4; if the reaction involves two $H_{fcc}$ species, the reaction mechanism includes surface diffusion of one adsorbed hydrogen from an fcc site to a neighboring top site before the two hydrogen atoms combine to liberate hydrogen gas. The transition state consists of a $H_2$ molecule with a slightly stretched H–H bond located on top of the metal surface. Hence, the Tafel reaction between two $H_{fcc}$ species is equivalent to that of $H_{fcc}$ + $H_{top}$ with an additional energetic penalty associated with surface diffusion.

# 5 Minimum energy pathway of Volmer reaction into fcc site

The top-hollow Volmer–Tafel mechanism in the main article includes a Volmer step into an empty fcc site to close the catalytic cycle. Figure S5 shows the potential-dependent minimum energy pathways of this process. Here, the reaction is exothermic for all potentials $U \leq 0$ $V_{SHE}$, and the reaction barrier is $\leq 0.19$ eV for $U \leq 0$ $V_{SHE}$. The inflection point at $x \sim 0.7$ on the relative reaction coordinate axis corresponds to hydrogen adsorption into a top site, followed by surface diffusion into the neighoring hollow site.

# 6 Elementary step electron transfer

The overall reaction to produce $H_2$ from two (bulk) solvated protons must consume precisely two electrons, and here we describe the detailed electron transfer mechanisms as inferred from these calculations. Structural optimization of metal–solvent interfaces with a surplus

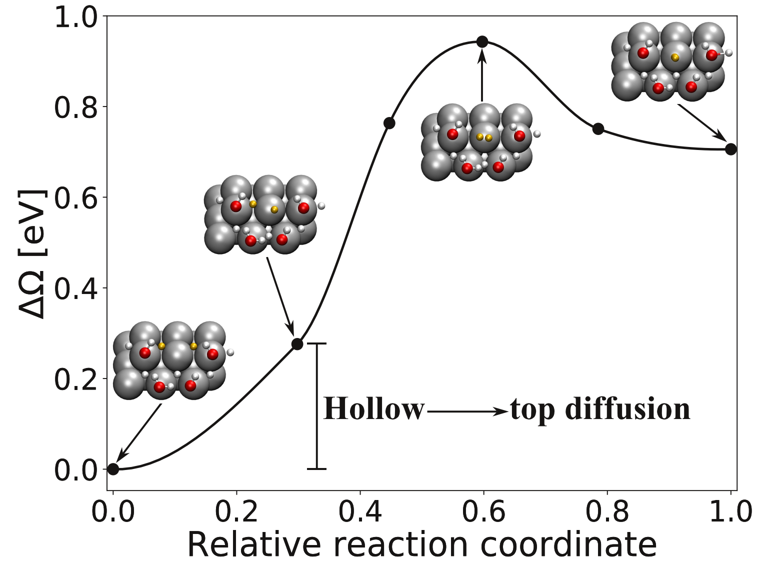


**Figure S4:** Minimum energy pathway of the Tafel reaction between two $H^*_{fcc}$ atoms. Note that the reaction proceeds in an equivalent way as the top–hollow mechanism, after diffusion of an $H_{fcc}$ into a top-site.

of hydrogen atoms induces a charge separation where a fractional number of electrons from the additional hydrogen atom transfers to the metal. As mentioned in the main article, we observe this behavior with both Bader charge analysis[5] and a grand canonical description (addition/subtraction of electrons).

With the Solvated Jellium approach, we "inject" electrons along the course of the reaction pathway in order to keep the potential constant. Intriguingly, we find that the greatest change in the number of excess electrons along the reaction trajectory always coincides with the transition state for the electrochemical reactions. (We previously found similar results for low-coverage Volmer reactions on both Au and Pt.[3]) These results, shown in Figure S6, indicate that the transition states correspond to the formation of Pt–H and H–H bonds for the Volmer and Heyrovsky reactions, respectively. Hence, the surface charge is depleted at the transition state, and electrons must be injected into the metal to keep the work function constant.

Figure S6 shows the minimum energy pathway and electron transfer of each elementary HER step at the equilibrium potential. As previously mentioned, the Volmer and Heyrovsky steps are electrochemical reactions, and thus exhibit significant charge transfer along the reaction trajectory. However, the charge transfer is less than unity; the charge transfer for the Volmer and Heyrovsky steps is 0.56e and 0.70e, respectively. Chen *et. al.*[4] attribute this fractional charge transfer to hybridization of the metal electrode and the protonated water bilayer when the additional proton is localized close to the interface. Hence, the initial states presented in this article are pseudo-initial states; that is, stable intermediates between the true initial state—a proton solvated in the bulk of the electrolyte—and the final state. However, these partial reaction pathways provide important mechanistic insight. The Volmer step at the equilibrium potential, shown in Figure S6a, is largely governed by unfavorable thermodynamics (approaching the linear region with a slope of unity in Figure 2 of the

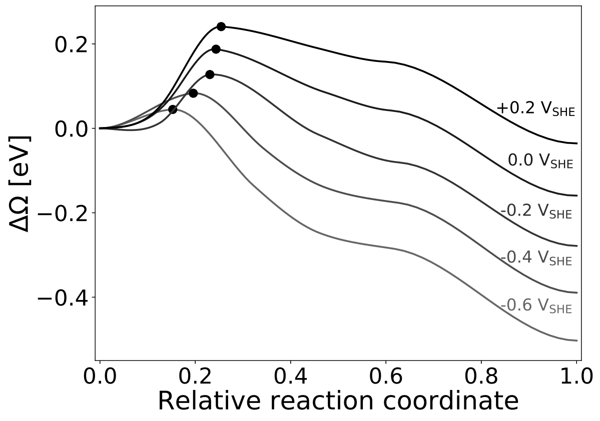


**Figure S5:** Minimum energy pathway of the Volmer reaction into an empty fcc site.

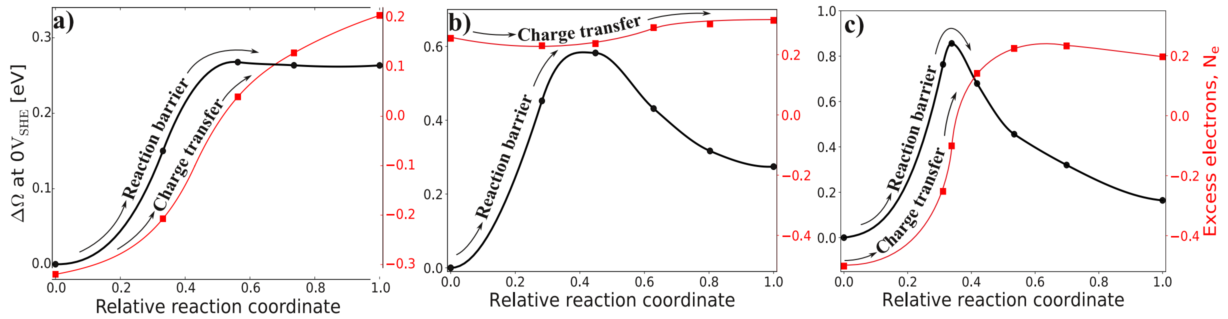


**Figure S6:** Minimum energy pathways (black circles) and electron transfer (red squares) of the a) Volmer, b) Tafel and c) Heyrovsky steps of HER at the equilibrium potential.

main article). The transition state of the Heyrovsky step, however, is relatively early along the reaction pathway, where the later part is hydrogen gas diffusion with negligible charge transfer. The minimum energy pathway profiles of these two reactions are thus significantly different. However, regardless of which elementary electrochemical reaction is studied, we find that the highest degree of electron transfer coincides with the transition state for the reaction. Therefore, we conclude that the Volmer and Heyrovsky transition states presented in this article correspond to the barriers associated with the electrochemical (charge transfer) reactions, and not any surface/$H_2$ diffusion events. At this level of theory, we can consider these concerted proton–electron transfers.

The Tafel step is a chemical surface reaction between two adsorbed hydrogen atoms. This phenomenon is captured in the simulation; the charge transfer required to hold the potential constant is negligible compared to the Volmer and Heyrovsky steps. As outlined in the main article, the overall reaction energy exhibits a slight potential dependence. We interpret the non-zero charge transfer of the Tafel reaction as a consequence of small changes in the surface dipole due to reorganization of the water bilayer. However, the overall charge transfer of the Tafel reaction (Figure S6b) is merely ~0.1e, compared to 0.56e and 0.70e for the Volmer and Heyrovsky reactions, respectively.

Interestingly, we find that the relationship between charge transfer and transition state location along the reaction coordinate is consistent over a wide range of potentials for the elementary electrochemical reactions; the transition state and electron transfer regions move concertedly along the reaction trajectory when the potential is varied. This trend is shown for the Volmer step in Figure S7 and indicates that the transition state geometry corresponds to metal charge depletion (Pt–H or H–H bond formation) over the entire potential range.

Figure S7 shows the minimum energy pathway (MEP) and electron transfer of the Volmer reaction at varying applied potentials. We observe concerted movement of the electron transfer and transition state along the reaction coordinate when the applied potential is varied; the inflection point of the electron transfer curve coincides with the transition state for all applied potentials. This indicates that the transition state corresponds to the formation of a metal-hydrogen bond over the entire voltage range. Hence, the metal charge is depleted at the transition state, and electrons must be injected into the electrode to keep the potential (work function) constant.

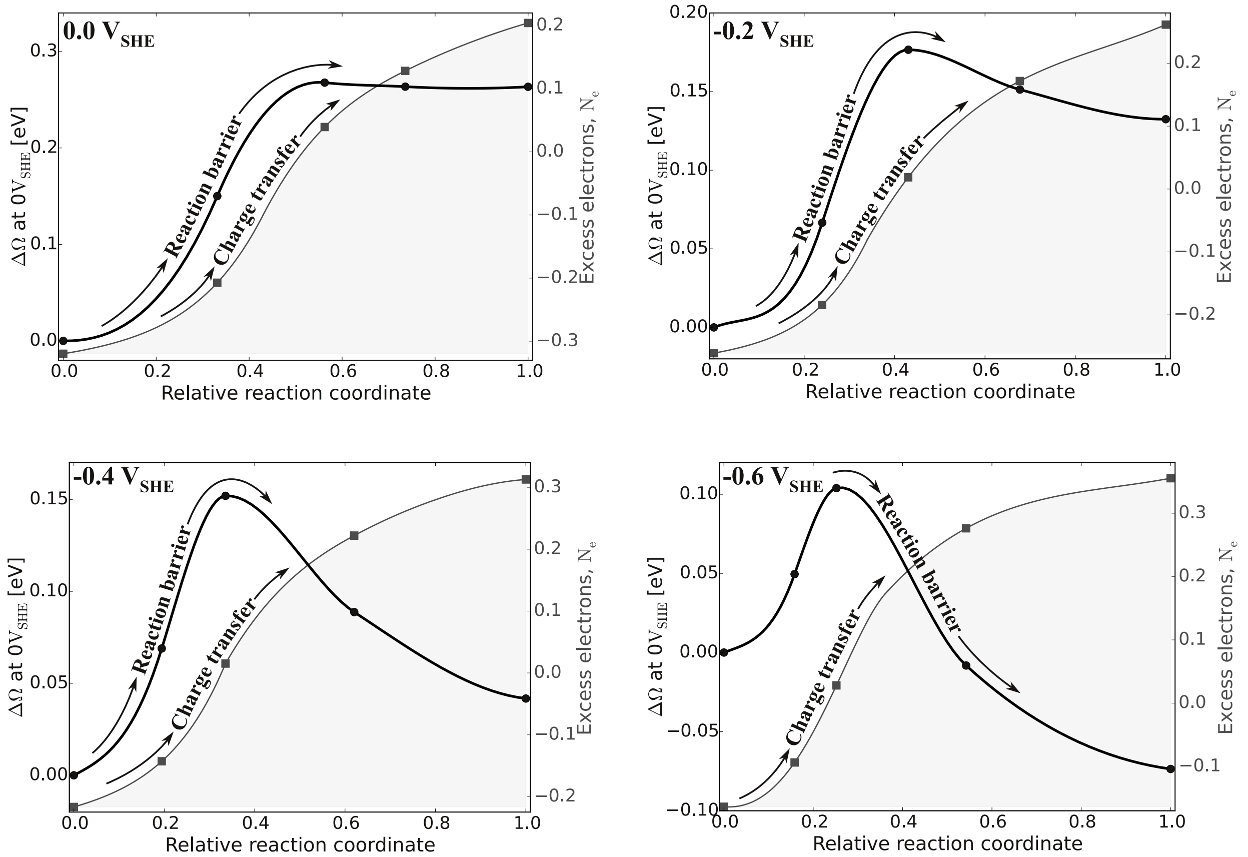


**Figure S7:** Minimum energy pathways (black circles) and charge transfer (gray squares) for the Volmer reaction on Pt(111) at varying potentials. Note that the inflection point of the electron transfer and transition state of the reaction pathway move concertedly with applied potential.

# 7 Microkinetic model

Here, we describe the details of the microkinetic model that the results in Figure 4 of the main article are based on. Each of the reaction mechanisms was studied with their own models and each of them will be described separately. However, there are steps in the reaction mechanisms that are common for all of them. We will discuss these steps first:

The first step in all reaction mechanisms is the diffusion of a proton from the electrolyte bulk to the electrode surface. This step consists of diffusion of the proton through the electrochemical double layer into the high field region. Since we do not expect a significant barrier from this process, we treat it as an equilibrated process. This reaction is shown below:

$$\text{(I): } \mathrm{H}^{+}_{(\mathrm{aq})} \xrightleftharpoons{K_\mathrm{I}} \mathrm{H}^{\mathrm{x}+}_{(\mathrm{if},(\mathrm{I}))},$$

where $K_\mathrm{I} = \exp\left(\frac{-\Delta G^r_\mathrm{I}}{k_\mathrm{B}T}\right)$ is the equilibrium constant of the diffusion step. Consequently, the activity of the protons at the interface can be defined as $a_{\mathrm{H^{x+}}_{\mathrm{if},(\mathrm{I})}} = a_{\mathrm{H}^+_{\mathrm{aq}}} K_\mathrm{I}$.

The Volmer reaction into a top site is the second step in common for all three mechanisms (Heyrovsky, top-hollow Tafel, top-top Tafel). The respective reaction is

$$(\mathrm{V_{top}})\text{: } \mathrm{H}^{\mathrm{x}+}_{\mathrm{if},(\mathrm{I})} + *_{\mathrm{top}} \underset{k_{\mathrm{V-top}}}{\overset{k_{\mathrm{Vtop}}}{\rightleftharpoons}} \mathrm{H}*_{\mathrm{top}}$$

where $*_{\mathrm{top}}$ refers to a free ontop binding site on the electrode's surface. The rate constants applied in this mechanism are

$$k_{\mathrm{V_{top}}} = \nu \exp\left(\frac{-\Delta G^{\ddagger}_{\mathrm{V_{top}}}}{k_\mathrm{B}T}\right), \tag{5}$$

and

$$k_{\mathrm{V_{-top}}} = \nu \exp\left(\frac{-\Delta G^{\ddagger}_{\mathrm{V_{-top}}}}{k_\mathrm{B}T}\right), \tag{6}$$

where the preexponential factor $\nu = \frac{k_\mathrm{B}T}{h} (\approx 10^{13}\ \mathrm{s}^{-1})$ was used throughout all the microkinetic models. $\Delta G^{\ddagger}_{\mathrm{V_{top}}}$ and $\Delta G^{\ddagger}_{\mathrm{V_{-top}}}$ are the activation free energies for the forward and backward reactions, respectively, as calculated from constant potential CI-NEB and shown in the free energy diagrams of the main article.

With these two processes in mind, we can build the detailed microkinetic models for the three studied reaction mechanisms.

## 7.1 Volmer–Heyrovsky mechanism

In addition to the first diffusion (I) and $\mathrm{V_{top}}$ steps, the Volmer-Heyrovsky mechanism includes solvation of a second proton followed by electrochemical liberation of $H_2$.

Since HER is a two electron-two proton transfer reaction, a second proton has to approach from the bulk of the solution. Similar to step (I), we describe this as an equilibrated process between the bulk solvated proton and the proton at the interface.

$$\text{(II): } \mathrm{H}^+_{(\mathrm{aq})} \xrightleftharpoons{K_{\mathrm{II}}} \mathrm{H}^{\mathrm{x}+}_{(\mathrm{if},(\mathrm{II}))},$$

with

$$K_{\mathrm{II}} = \exp\left(\frac{-\Delta G^r_{\mathrm{II}}}{k_{\mathrm{B}}T}\right) \tag{7}$$

Although the reaction looks almost identical to (I), we found that $\Delta G^r_{\mathrm{II}}$ is slightly higher than $\Delta G^r_{\mathrm{I}}$. The reason for this difference is that the proton approaching the surface already positions itself next to the top-adsorbed H* from the $\mathrm{V_{top}}$ step. The presence of the $\mathrm{H_{top}}$ species changes the equilibrium slightly and makes it necessary to treat this diffusion step explicitly.

Diffusion step (II) is followed by the Heyrovsky reaction:

$$\text{(Hey): } \mathrm{H}^{\mathrm{x}+}_{(\mathrm{if},(\mathrm{II}))} + *\mathrm{H_{top}} \underset{k_{-\mathrm{Hey}}}{\overset{k_{\mathrm{Hey}}}{\rightleftharpoons}} \mathrm{H}_{2(\mathrm{g})} + *_{\mathrm{top}},$$

with

$$k_{\mathrm{Hey}} = \nu \exp\left(\frac{-\Delta G^{\ddagger}_{\mathrm{Hey}}}{k_{\mathrm{B}}T}\right), \tag{8}$$

and

$$k_{-\mathrm{Hey}} = \nu \exp\left(\frac{-\Delta G^{\ddagger}_{-\mathrm{Hey}}}{k_{\mathrm{B}}T}\right), \tag{9}$$

being the rate constants of the forward and backward reaction, respectively, including the corresponding activation free energies $\Delta G^{\ddagger}_{\mathrm{Hey}}$ and $\Delta G^{\ddagger}_{-\mathrm{Hey}}$. Since $\Delta G^{\ddagger}_{-\mathrm{Hey}}$ is substantially higher than $\Delta G^{\ddagger}_{\mathrm{Hey}}$, we treat this as an irreversible reaction. Hence, we neglect the backwards reaction.

Based on the reactions above, the coverage ($\theta_{\mathrm{top}}$) of the top sites of the electrode can be calculated by either integrating

$$\frac{d\theta_{\mathrm{top}}}{dt} = k_{\mathrm{V_{top}}} a_{\mathrm{H}^{\mathrm{x}+}_{\mathrm{if},(\mathrm{I})}} (1 - \theta_{\mathrm{top}}) - k_{\mathrm{V_{-top}}} \theta_{\mathrm{top}} - k_{\mathrm{Hey}} \theta_{\mathrm{top}} a_{\mathrm{H}^{\mathrm{x}+}_{\mathrm{if},(\mathrm{II})}} \tag{10}$$

until a steady state is reached or by deriving an analytical expression for $\theta_{top}$ via a pseudo steady state approximation.

Finally, the reaction rate [site$^{-1}$ s$^{-1}$] and current density can be calculated as shown below.

$$r_{\mathrm{Hey}} = k_{\mathrm{Hey}} \theta_{\mathrm{top}} a_{\mathrm{H}^{\mathrm{x}+}_{\mathrm{if},(\mathrm{II})}} \tag{11}$$

and

$$j_{\mathrm{Hey}} = n_e e C_s r_{\mathrm{Hey}}, \tag{12}$$

where $n_e$=2 is the number of electrons transferred, $e$ is the elementary charge and $C_s$ is the site density on the electrode.

## 7.2 Top-hollow Volmer–Tafel

Other than (I) and ($V_{top}$), the reactions characteristic of the top-hollow Volmer–Tafel route are the Tafel reaction (T), a second proton approaching the interface region from the solvent bulk (III) and the second hydrogen adsorption step ($V_{fcc}$), where the latter recovers $H_{fcc}$ (complete fcc-hollow monolayer) of the electrode. (III) differs slightly from (I) and (II), since it represents diffusion from the solvent to an interface that has an fcc-hollow site vacancy. Surprisingly, this vacancy reduced the entropic penalty substantially, and thus the step has to be regarded separately.

The corresponding reactions characteristic for the top-hollow Tafel reaction are

$$\text{(T)}: *\,\mathrm{H_{top}} + *\mathrm{H_{fcc}} \underset{k_{-\mathrm{T}}}{\overset{k_{\mathrm{T}}}{\rightleftharpoons}} \mathrm{H_{2(g)}} + *_{\mathrm{fcc}} + *_{\mathrm{top}},$$

$$\text{(III)}: \mathrm{H^+_{(aq)}} \overset{K_{\mathrm{III}}}{\rightleftharpoons} \mathrm{H^{x+}_{(if,(III))}},$$

and

$$(\mathrm{V_{fcc}}): \mathrm{H^{x+}_{if,(II)}} + *_{\mathrm{fcc}} \underset{k_{\mathrm{V-fcc}}}{\overset{k_{\mathrm{Vfcc}}}{\rightleftharpoons}} \mathrm{H}*_{\mathrm{fcc}}\ ,$$

where the actual order of the described reactions is secondary in the microkinetic model, since the rate equations are unchanged.

In this process, we account for the two adsorption sites separately, since the energetics of the Volmer reaction are significantly different. Hence, two equations are required to define the coverages of the fcc-hollow and top sites. These equations are shown below.

$$\frac{d\theta_{\mathrm{fcc}}}{dt} = k_{\mathrm{V_{fcc}}} a_{\mathrm{H^{x+}_{if,(III)}}} (1-\theta_{\mathrm{fcc}}) - k_{\mathrm{V_{-fcc}}}\theta_{\mathrm{fcc}} - k_{\mathrm{T}}\theta_{\mathrm{fcc}}\theta_{\mathrm{top}} \tag{13}$$

and

$$\frac{d\theta_{\mathrm{top}}}{dt} = k_{\mathrm{V_{top}}} a_{\mathrm{H^{x+}_{if,(I)}}} (1-\theta_{\mathrm{top}}) - k_{\mathrm{V_{-top}}}\theta_{\mathrm{top}} - k_{\mathrm{T}}\theta_{\mathrm{top}}\theta_{\mathrm{fcc}} \tag{14}$$

The equations can be solved numerically or analytically via a pseudo steady state approximation.

After reaching steady state for both coverages, the rate of the Tafel reaction can be calculated as

$$r_{\mathrm{T}} = k_{\mathrm{T}}\theta_{\mathrm{top}}\theta_{\mathrm{fcc}}, \tag{15}$$

where the Tafel step is treated as irreversible due to the significant reaction barrier of the backwards reaction. Finally, the current density $j_{\mathrm{T}}$ can be calculated by substituting $r_{\mathrm{Hey}}$ by $r_{\mathrm{T}}$ in equation 12.

As a final remark, it should be noted that we assume surface diffusion between sites of the same type to be fast and thermoneutral. As consequence, we do not explicitly account for the fact that the two protons involved in the Tafel reaction need to be in neighboring sites.

### 7.3 Top-top Volmer–Tafel

The final process under study is the top-top Volmer–Tafel mechanism. This has been identified as a viable route for HER, especially at increasingly negative potentials.

The reaction steps in this mechanism differ from the top-hollow Volmer–Tafel mechanism in that both protons involved in the Tafel step are $H_{top}$ species adsorbed in top sites. As a consequence, the mechanism has its own characteristic reaction, namely

$$\text{(T2): } *\mathrm{H}_{\mathrm{top}} + *\mathrm{H}_{\mathrm{top}} \underset{k_{-\mathrm{T}}}{\overset{k_{\mathrm{T}}}{\rightleftharpoons}} \mathrm{H}_{2(\mathrm{g})} + 2*_{\mathrm{top}},$$

In the definition of the rate equation, we apply the same approximation as for the $H_{fcc}$ adsorption in the top-hollow Volmer–Tafel mechanism; the adsorption energy of H in the top sites is independent of the current top-site coverage. Then, the coverage can be calculated via

$$\frac{d\theta_{\mathrm{top}}}{dt} = k_{\mathrm{V_{top}}} a_{\mathrm{H}^{x+}_{\mathrm{if,(I)}}} (1 - \theta_{\mathrm{top}}) - k_{\mathrm{V_{-top}}} \theta_{\mathrm{top}} - k_{\mathrm{T2}} \theta_{\mathrm{top}}^2, \quad (16)$$

where $k_{\mathrm{T2}} = \nu \exp\left(-\frac{\Delta G^{\ddagger}_{\mathrm{T2}}}{k_{\mathrm{B}} T}\right)$ is the rate constant of the top-top Tafel reaction.

The resulting rate [site$^{-1}$ s$^{-1}$] of the reaction for this mechanism is

$$r_{\mathrm{T2}} = k_{\mathrm{T2}} \theta_{\mathrm{top}}^2 \quad (17)$$

and the resulting current density can be retrieved via equation 12, where $r_{T2}$ is the relevant rate.

### 7.4 Potential dependence

In order to include potential dependence into the microkinetic analyses, microkinetic models for a large sample of potentials in the range of interest were created. The applied potential affects the free energies of all electrochemical steps in the model, as shown in the free energy diagrams in the main article. In order to obtain smooth curves, the relevant free energies were fitted by linear functions for reaction and potential-independent activation free energies, and by $\frac{(\Delta E + 4b)^2}{16b}$ for transition states of electrochemical elementary steps.

## 8 Interpretation of Tafel slopes

The Tafel slopes presented in the manuscript are the direct outputs of the complete, thermodynamically consistent microkinetic model described above; no kinetic assumptions of rate-limiting steps or equilibrated reactions were employed. Here, we employ various assumptions about rate-limiting steps and the Tafel slopes that result, in order to interpret the Tafel slopes provided by the microkinetic model.

We first derive a general understanding of the intuitive picture of Tafel slopes, before going into each possible mechanism individually. Assume the hydrogen-liberating step is

**Table S1:** Linear and parabolic fits for the reaction and activation free energies used in microkinetic models.

| | $\Delta G_{\rm IS}(U_{\rm SHE})$ | $\Delta G_{\rm TS}(U_{\rm SHE})$ | $\Delta G_{\rm FS}(U_{\rm SHE})$ |
|---|---|---|---|
| | | All mechanisms | |
| (I) | 0 | - | $0.367U_{\rm SHE}$ + 0.185 |
| ($V_{\rm top}$) | $0.367U_{\rm SHE}$ + 0.185 | $\Delta G^r$= $0.587U_{\rm SHE}$ + 0.216, b= 0.101 | $0.954U_{\rm SHE}$ + 0.401 |
| | | Volmer-Heyrovsky | |
| (II) | $0.954U_{\rm SHE}$ + 0.401 | - | $1.162U_{\rm SHE}$ + 0.610 |
| (H) | $1.162U_{\rm SHE}$ + 0.610 | $\Delta G^r$= $0.838U_{\rm SHE}$ - 0.610, b= 0.938 | $2.000U_{\rm SHE}$ |
| | | Top-hollow Volmer-Tafel | |
| (T) | $0.954U_{\rm SHE}$ + 0.401 | $0.909\mathrm{U}_{\rm SHE}$ + 0.941 | $1.006U_{\rm SHE}$ + 0.110 |
| (III) | $1.006U_{\rm SHE}$ + 0.110 | - | $1.433U_{\rm SHE}$ + 0.157 |
| ($V_{\rm fcc}$) | $1.433U_{\rm SHE}$ + 0.157 | $\Delta G^r$= $0.567U_{\rm SHE}$ - 0.157, b= 0.237 | $2.000U_{\rm SHE}$ |
| | | Top-top Volmer-Tafel | |
| (T2) | $1.880U_{\rm SHE}$ + 0.861 | $1.862U_{\rm SHE}$ + 1.144 | $2.000U_{\rm SHE}$ |

rate-limiting and can occur by any of three mechanisms:

$$\mathrm{H}{*} + \mathrm{H}{*} \longrightarrow \mathrm{H_2} + 2{*} \qquad \text{(top–top Tafel)}$$

$$\mathrm{H}{*} + \mathrm{H}{\circ} \longrightarrow \mathrm{H_2} + {*} + {\circ} \qquad \text{(top–hollow Tafel)}$$

$$\mathrm{H}{*} + \mathrm{H^+} + \mathrm{e^-} \longrightarrow \mathrm{H_2} + {*} \qquad \text{(top Heyrovsky)}$$

where $*$ and $\circ$ are used to distinguish top and hollow adsorption sites, respectively. The transition-state theory rate is rigorously expressed with respect to activities of the reactants:

$$r = k^{\ddagger} a_1 a_2 \tag{18}$$

where $k^{\ddagger} = (k_{\rm B}T/h)e^{-\Delta G^{\ddagger}/k_{\rm B}T}$. In the case of Heyrovsky, $a_2$ is the proton activity, which is dictated by the pH and therefore constant. The coverages can be assumed to be quasi-equilibrated via the Volmer step:

$$\frac{a_{\rm H*}}{a_* \, a_{\rm H^+}} = \exp\left\{\frac{-\Delta G^{\circ}_{\text{Volmer-top}}}{k_{\rm B}T}\right\} \equiv K_{\text{Volmer-top}}$$

and identical for the Volmer–hollow step. Note that we do *not* make this assumption in the microkinetic model. However, we observe equilibrium behavior in the microkinetic model, thus validating this assumption here. Note that the free energy change of this reaction is directly dependent upon the voltage via $eU$. The activity of H$*$ can be assumed to be nearly directly proportional to the coverage of H $\theta_{\rm H}$, while the activity of vacant sites can be assumed to be nearly directly proportional to $(1-\theta_{\rm H})$. Therefore, when hydrogen coverage is low, $a_* \sim 1$ and $a_{\rm H*}$ varies exponentially with potential, thus, giving an exponential change in the reaction rate $r$. Conversely, when hydrogen coverage is of order 1, $a_{\rm H*}$ varies little with potential, as the surface is saturated; the equilibrium ratio is held constant by exponential changes in $a_*$, which is very low.

Equivalently, we can say when $a_{\mathrm{H}*}$ is low,

$$a_{\mathrm{H}*} \propto \exp\left\{\frac{-\Delta G^{\circ}_{\text{Volmer-top}}}{k_{\mathrm{B}}T}\right\}$$

since $a_* \sim 1$, but when $a_{\mathrm{H}*}$ is high,

$$a_{\mathrm{H}*} \propto 1$$

This treatment is general to hydrogen binding in either site. Thus, when hydrogen coverages are low, equation (18) can be written as

$$r \propto \exp\left\{\frac{-\left(\Delta G^{\ddagger} + \Delta G^{\circ}_1 + \Delta G^{\circ}_2\right)}{k_{\mathrm{B}}T}\right\} \tag{19}$$

where $\Delta G^{\circ}_1$ and $\Delta G^{\circ}_2$ are the reaction free energy changes corresponding to $a_1$ and $a_2$. If the coverage corresponding to either $a_1$ or $a_2$ becomes high (order one), the associated free energy drops out of equation (19). Similarly, the activity corresponding to pH in the Heyrovsky mechanism does not have a free energy term entering equation (19), since no equilibration step is necessary.

From equation (19), the conclusions on Tafel slopes reached in the text are straightforward.

As outlined in the main article, Tafel slopes of 120, 40 and 30 mV dec$^{-1}$ are associated with rate-limiting Volmer, Heyrovsky and Tafel steps, respectively. Here, we derive the experimentally observed Tafel slopes of HER from transition state theory and microkinetic models.

## 8.1 Volmer

The Volmer reaction is a proton-coupled electron transfer step to form adsorbed hydrogen, as shown in equation 20

$$* + \left(\mathrm{H}^+ + \mathrm{e}^-\right) \xrightarrow{\mathrm{k}} \mathrm{H}*. \tag{20}$$

If the Volmer reaction is rate-limiting, the rate can be expressed as

$$r = k\,(1-\theta)\,a_{\mathrm{H}^+}, \tag{21}$$

where $a_{\mathrm{H}^+}$ is the proton activity (unity at pH=0) and $\theta$ is the hydrogen coverage. The rate can be converted to current density as shown below

$$j = n_e \cdot e \cdot k\,(1-\theta)\,a_{\mathrm{H}^+} \cdot C_S, \tag{22}$$

where $n_e$ and $C_S$ are the number of electrons involved and the total concentration of surface sites, respectively, and $e$ is the positive elementary charge.

The rate constant, k, in equation 22 comes from transition state theory

$$k = \frac{k_{\mathrm{B}}T}{h} \exp\left(-\frac{\Delta G^{\ddagger}}{k_{\mathrm{B}}T}\right), \tag{23}$$

where $\Delta G^{\ddagger}$ is the free energy reaction barrier of the rate-determining elementary step. Hence, the complete expression for the current density is

$$j = n_e \cdot e \cdot \frac{k_{\mathrm{B}}T}{h} \exp\left(-\frac{\Delta G^{\ddagger}}{k_{\mathrm{B}}T}\right)(1-\theta)\, a_{\mathrm{H}^+} \cdot C_S. \tag{24}$$

In order to calculate the Tafel slope, the current density must be converted into a log scale.

$$\begin{aligned} \log_{10} j &= \log_{10}(n_e) + \log_{10}(e) + \log_{10}(k) + \log_{10}\left((1-\theta)a_{\mathrm{H}^+}\right) = \\ &= \log_{10}(n_e \cdot e\frac{k_{\mathrm{B}}T}{h}a_{\mathrm{H}^+}) + \log_{10}\left(\exp\left(-\frac{\Delta G^{\ddagger}}{k_{\mathrm{B}}T}\right)\right) + \log_{10}\left(1-\theta\right). \end{aligned} \tag{25}$$

Equation 25 can be simplified further:

$$\log_{10} j = \log_{10}(n_e \cdot e\frac{k_{\mathrm{B}}T}{h}a_{\mathrm{H}^+}) - \frac{\Delta G^{\ddagger}}{2.303k_{\mathrm{B}}T} + \log_{10}\left(1-\theta\right), \tag{26}$$

where the potential dependence of the coverage term, $\log_{10}(1-\theta)$, is neglected for low driving forces, since the term is essentially constant. In a subsequent section, we show a complete derivation of the potential-dependent coverage for the top-hollow Tafel mechanism. The free energy activation energy can be expressed as a combination of the standard free energy reaction energy and an additional overpotential term

$$\Delta G^{\ddagger} = \Delta G^{\circ\ddagger} - \beta e \eta, \tag{27}$$

where $\beta$ is the symmetry factor ($0 \leq \beta \leq 1$), e is the (positive) elementary charge and $\eta$ is the overpotential. Equations 26 and 27 yield the following expression for the free energy reaction barrier

$$\Delta G^{\ddagger} = \Delta G^{\circ\ddagger} - \beta e \eta = log_{10}(n_e\ \frac{k_{\mathrm{B}}T}{h}a_{\mathrm{H}^+}) - \frac{\Delta G^{\circ\ddagger}}{2.303k_{\mathrm{B}}T} + \frac{\beta e \eta}{2.303k_{\mathrm{B}}T}, \tag{28}$$

where only the final term is potential-dependent. Hence, the partial derivative of the logarithm of the current density with respect to overpotential yields a single term,

$$\frac{\partial log_{10}\ j}{\partial \eta} = \frac{\beta e}{2.303k_{\mathrm{B}}T}. \tag{29}$$

Inverting equation 29 yields the Tafel slope:

$$\frac{\partial \eta}{\partial log_{10}\ j} = \frac{2.303k_{\mathrm{B}}T}{\beta e} = \frac{59.2\mathrm{mV}}{\beta e}, \tag{30}$$

at 298 K. If one assumes a symmetry factor of 0.5, the Tafel slope of a rate-limiting Volmer step is

$$\frac{\partial \eta}{\partial log_{10}\ j} = \frac{59.2\text{mV}}{0.5e} \approx 120 \text{ mV dec}^{-1}. \tag{31}$$

## 8.2 Heyrovsky

The Heyrovsky reaction is an electrochemical elementary step between a proton-electron pair and an adsorbed hydrogen atom. This step is always preceded by a proton discharge step to form adsorbed hydrogen, *i.e.* the Volmer reaction. If the Heyrovsky reaction is rate-limiting, the Volmer reaction is relatively fast and can be assumed to be equilibrated (pseudo steady-state approximation (PSSA)):

$$* + \left(\text{H}^+ + \text{e}^-\right) \underset{k_{-\text{V}}}{\overset{k_\text{V}}{\rightleftharpoons}} \text{H}*, \tag{32}$$

$$\theta = K_\text{V}\left(1-\theta\right) a_{\text{H}^+}, \tag{33}$$

where the equilibrium constant, $K_\text{V}$, is calculated from the overall reaction energy

$$K_\text{V} = \exp\left(-\frac{\Delta G^r_\text{V}}{k_\text{B}T}\right). \tag{34}$$

The Heyrovsky reaction involves a proton-electron pair and the adsorbed hydrogen atom from the preceding Volmer step.

$$\left(\text{H}^+ + \text{e}^-\right) + \text{H}* \xrightarrow{k_\text{H}} \text{H}_2 + *. \tag{35}$$

The reaction rate is calculated from this irreversible and rate-limiting step

$$r = k_\text{H} \cdot \theta \cdot a_{\text{H}^+}, \tag{36}$$

where the expression for $\theta$ in equation 33 can be substituted into equation 36:

$$r = k_\text{H} K_\text{V}\left(1-\theta\right) a^2_{\text{H}^+}. \tag{37}$$

Now, we substitute the transition state theory rate constant expression from equation 23 and the Volmer equilibrium constant expression (equation 34) into equation 37.

$$r = \frac{k_\text{B}T}{h}\left(1-\theta\right) a^2_{\text{H}^+} \exp\left(-\frac{\Delta G^\ddagger_\text{H} + \Delta G^r_\text{V}}{k_\text{B}T}\right) = \frac{k_\text{B}T}{h}\left(1-\theta\right) a^2_{\text{H}^+} \exp\left(-\frac{\Delta G^\ddagger}{k_\text{B}T}\right). \tag{38}$$

where $\Delta G^\ddagger$ is the net reaction barrier from the initial Volmer step to the rate-limiting Heyrovsky step. The rate expression in equation 38 is then converted to current density as shown below.

$$j = \frac{k_\text{B}T}{h} n_e e C_S \left(1-\theta\right) a^2_{\text{H}^+} \exp\left(-\frac{\Delta G^\ddagger}{k_\text{B}T}\right). \tag{39}$$

where $C_S$ and $n_e$ are the number of available surface sites and number of electrons involved in the reaction, respectively. Now, we can separate the net reaction barrier into standard free energies and overpotential contributions

$$\Delta G^{\ddagger} = \Delta G^{\ddagger}_{\mathrm{H}} + \Delta G^{r}_{\mathrm{V}} = \Delta G^{\circ\ddagger}_{\mathrm{H}} + \Delta G^{\circ r}_{\mathrm{V}} - \eta e \beta_{\mathrm{H}} - \eta e = \Delta G^{\circ\ddagger} - (1 + \beta_{\mathrm{H}})\, \eta e, \tag{40}$$

and the final expression for the current density is thus

$$j = \frac{k_{\mathrm{B}}T}{h} n_e e C_S \,(1-\theta)\, a^2_{\mathrm{H}^+} \exp\left(-\frac{\Delta G^{\circ\ddagger} - (1+\beta_{\mathrm{H}})\,\eta e}{k_{\mathrm{B}}T}\right). \tag{41}$$

Now, the current density is converted to a log scale

$$\log_{10} j = \log_{10}\left(\frac{k_{\mathrm{B}}T}{h} n_e e C_S \,(1-\theta)\, a^2_{\mathrm{H}^+}\right) + \frac{-\Delta G^{\circ\ddagger} + (1+\beta_{\mathrm{H}})\,\eta e}{2.303 k_{\mathrm{B}}T}. \tag{42}$$

The partial derivative of the logarithm of current density with respect to overpotential yields only one term, since $\log_{10}(1-\theta)$ in equation 42 is essentially independent of the applied potential.

$$\frac{\partial \log_{10} j}{\partial \eta} = \frac{(1+\beta_{\mathrm{H}})\, e}{2.303 k_{\mathrm{B}}T}. \tag{43}$$

The Tafel slope is obtained by inverting the expression in equation 43:

$$\frac{\partial \eta}{\partial \log_{10} j} = \frac{2.303 k_{\mathrm{B}}T}{(1+\beta_{\mathrm{H}})\, e} = \frac{59.2\mathrm{mV}}{(1+\beta_{\mathrm{H}})\, e}, \tag{44}$$

If one assumes a Heyrovsky symmetry factor of 0.5, the Tafel slope is approximately 40 mV dec$^{-1}$

$$\frac{\partial \eta}{\partial \log_{10} j} = \frac{59.2\mathrm{mV}}{(1+\beta_{\mathrm{H}})\, e} = \frac{59.2\mathrm{mV}}{(1+0.5)\, e} \approx 40 \text{ mV dec}^{-1}. \tag{45}$$

## 8.3 Top-top Tafel

This reaction mechanism is characterized by a rate-limiting Tafel step, which is preceded by two Volmer reactions. The hydrogen coverage is dependent on the Volmer reactions, as shown in equation 33

$$\theta = K_{\mathrm{V}}\,(1-\theta)\, a_{\mathrm{H}^+} \text{ (PSSA)}. \tag{46}$$

The characteristic equation for the rate-limiting Tafel step is

$$2\mathrm{H}* \xrightarrow{k_{\mathrm{T}}} \mathrm{H}_2 + 2*, \tag{47}$$

and the rate equation is

$$r = k_{\mathrm{T}}\theta^2 = k_{\mathrm{T}}\left(K_{\mathrm{V}}\,(1-\theta)\, a_{\mathrm{H}^+}\right)^2. \tag{48}$$

Now, we collect the equilibrium constants from the Volmer reactions and the rate constant for the Tafel reaction

$$k_{\mathrm{T}} K_{\mathrm{V}}^{2} = \frac{k_{\mathrm{B}} T}{h} \exp\left(-\frac{\Delta G_{\mathrm{T}}^{\ddagger}}{k_{\mathrm{B}} T}\right) \exp\left(-\frac{2\Delta G_{\mathrm{V}}^{r}}{k_{\mathrm{B}} T}\right) = \frac{k_{\mathrm{B}} T}{h} \exp\left(-\frac{2\Delta G_{\mathrm{V}}^{r} + \Delta G_{\mathrm{T}}^{\ddagger}}{k_{\mathrm{B}} T}\right). \tag{49}$$

Following the steps in subsequent sections, we can convert the rate into current density, and the current density into a log scale

$$\log_{10} j = \log_{10}\left(\frac{k_{\mathrm{B}} T}{h} n_{e} e \left(1-\theta\right)^{2} a_{\mathrm{H}^{+}}^{2}\right) - \frac{2\Delta G_{\mathrm{V}}^{r} + \Delta G_{\mathrm{T}}^{\ddagger}}{2.303 k_{\mathrm{B}} T}, \tag{50}$$

where the first term is independent of applied potential in the low coverage limit. Now, we expand the reaction free energy and barrier into standard and potential-dependent terms

$$2\Delta G_{\mathrm{V}}^{r} + \Delta G_{\mathrm{T}}^{\ddagger} = 2\Delta G_{\mathrm{V}}^{\circ r} + \Delta G_{\mathrm{T}}^{\circ\ddagger} - \beta_{\mathrm{T}} e\eta - 2e\eta. \tag{51}$$

The final expression for the logarithm of the current density is thus

$$\log_{10} j = \log_{10}\left(\frac{k_{\mathrm{B}} T}{h} n_{e} e \left(1-\theta\right)^{2} a_{\mathrm{H}^{+}}^{2}\right) - \frac{2\Delta G_{\mathrm{V}}^{\circ r} + \Delta G_{\mathrm{T}}^{\circ\ddagger} - \beta_{\mathrm{T}} e\eta - 2e\eta}{2.303 k_{\mathrm{B}} T}, \tag{52}$$

and the Tafel slope is

$$\frac{\partial \eta}{\partial \log_{10} j} = \frac{2.303 k_{\mathrm{B}} T}{2e + \beta_{\mathrm{T}} e} \tag{53}$$

where $\beta_{\mathrm{T}}$=0 since the Tafel step is a chemical reaction. Hence, the Tafel slope is exactly 30 mV dec$^{-1}$

$$\frac{\partial \eta}{\partial \log_{10} j} = \frac{2.303 k_{\mathrm{B}} T}{2e} = 30 \text{ mV dec}^{-1}. \tag{54}$$

## 8.4 Top-hollow Tafel

Similar to the top-top Tafel route, this mechanism is characerized by a rate-limiting Tafel step that is preceded by two Volmer reactions. However, the hydrogen atoms involved in the Tafel reaction have different adsorption sites; one is adsorbed in a top site, whereas the other is adsorbed in an fcc-hollow site. Here, we distinguish between the top and hollow site coverages, as shown in equations 56 and 55.

$$\theta_{\mathrm{fcc}} = K_{\mathrm{fcc}} \left(1-\theta_{\mathrm{fcc}}\right) a_{\mathrm{H}^{+}} \tag{55}$$

$$\theta_{\mathrm{top}} = K_{\mathrm{top}} \left(1-\theta_{\mathrm{top}}\right) a_{\mathrm{H}^{+}}. \tag{56}$$

The reaction rate is a function of these two coverages

$$r = k_{\mathrm{T}}\theta_{\mathrm{top}}\theta_{\mathrm{fcc}} = k_{\mathrm{T}}K_{\mathrm{top}}K_{\mathrm{fcc}}\left(1-\theta_{\mathrm{top}}\right)\left(1-\theta_{\mathrm{fcc}}\right)a_{\mathrm{H}^+}^2. \tag{57}$$

As shown in previous sections, the reaction rate can be converted to current density

$$j = r \cdot n_e \cdot e \cdot C_S, \tag{58}$$

where the expression for the rate constant can be expanded to include reaction energies and barriers

$$j = \frac{k_{\mathrm{B}}T}{h}\left(1-\theta_{\mathrm{top}}\right)\left(1-\theta_{\mathrm{fcc}}\right)a_{\mathrm{H}^+}^2 n_e e C_S \exp\left(-\frac{\Delta G_{\mathrm{fcc}}^r + \Delta G_{\mathrm{top}}^r + \Delta G_{\mathrm{T}}^{\ddagger}}{k_{\mathrm{B}}T}\right), \tag{59}$$

and the logarithm of the current density is

$$\log_{10} j = \log_{10}\left(\frac{k_{\mathrm{B}}T}{h}\left(1-\theta_{\mathrm{top}}\right)a_{\mathrm{H}^+}^2 n_e e C_S\right) + \log_{10}\left(1-\theta_{\mathrm{fcc}}\right) + \log_{10}\exp\left(-\frac{\Delta G_{\mathrm{fcc}}^r + \Delta G_{\mathrm{top}}^r + \Delta G_{\mathrm{T}}^{\ddagger}}{k_{\mathrm{B}}T}\right). \tag{60}$$

In the top-top Tafel and Heyrovsky mechanisms, we treat the coverage as potential-independent; for low overpotentials the coverage is close to zero, and the term $\log_{10}(1-\theta)$ is essentially constant. In the top-hollow Tafel mechanism, however, the fcc-hollow coverage changes dramatically for the potentials of interest, *i.e.* at or around the equilibrium potential. Therefore, we explicitly include potential dependence of the fcc-hollow site coverage. The partial derivative of the logarithm of current density with respect to overpotential thus includes two terms

$$\frac{\partial \log_{10} j}{\partial \eta} = \frac{\partial \log_{10}\left(1-\theta_{\mathrm{fcc}}\right)}{\partial \eta} + \frac{\partial \log_{10}\left(\exp\left(-\frac{\Delta G_{\mathrm{fcc}}^r + \Delta G_{\mathrm{top}}^r + \Delta G_{\mathrm{T}}^{\ddagger}}{k_{\mathrm{B}}T}\right)\right)}{\partial \eta}. \tag{61}$$

From equation 55, we know that the coverage is a function of the equilibrium constant

$$\frac{\theta_{\mathrm{fcc}}}{1-\theta_{\mathrm{fcc}}} = K_{\mathrm{fcc}} = \exp\left(-\frac{\Delta G_{\mathrm{fcc}}^{\circ r} - e\eta}{k_{\mathrm{B}}T}\right). \tag{62}$$

Now, we rearrange the expression in equation 62 and solve explicitly for $\theta_{\mathrm{fcc}}$

$$\theta_{\mathrm{fcc}} = \frac{\exp\left(-\frac{\Delta G_{\mathrm{fcc}}^{\circ r} - e\eta}{k_{\mathrm{B}}T}\right)}{1 + \exp\left(-\frac{\Delta G_{\mathrm{fcc}}^{\circ r} - e\eta}{k_{\mathrm{B}}T}\right)}, \tag{63}$$

and

$$1-\theta_{\mathrm{fcc}} = \frac{1}{1 + \exp\left(-\frac{\Delta G_{\mathrm{fcc}}^{\circ r} - e\eta}{k_{\mathrm{B}}T}\right)}. \tag{64}$$

Equation 64 is then used with equation 61 to evaluate the partial derivative of the logarithm of current density with respect to overpotential. Here, we start by evaluating the

second term in equation 61

$$\left.\frac{\partial \log_{10} j}{\partial \eta}\right|_{\log_{10}(1-\theta_{\mathrm{fcc}})=\mathrm{constant}} = \frac{\partial \log_{10}\left(\exp\left(-\frac{\Delta G^{r}_{\mathrm{fcc}}+\Delta G^{r}_{\mathrm{top}}+\Delta G^{\ddagger}_{\mathrm{T}}}{k_{\mathrm{B}}T}\right)\right)}{\partial \eta}, \tag{65}$$

where separation of standard free energies and contributions from the overpotential leads to

$$\left.\frac{\partial \log_{10} j}{\partial \eta}\right|_{\log_{10}(1-\theta_{\mathrm{fcc}})=\mathrm{constant}} = \frac{\partial \log_{10}\left(\exp\left(-\frac{\Delta G^{\circ r}_{\mathrm{fcc}}+\Delta G^{\circ r}_{\mathrm{top}}+\Delta G^{\circ\ddagger}_{\mathrm{T}}-2e\eta-\beta_{\mathrm{T}}e\eta}{k_{\mathrm{B}}T}\right)\right)}{\partial \eta}. \tag{66}$$

This partial derivative is identical to that of the top-top Tafel mechanism; the symmetry factor is zero (chemical reaction), and only the potential-dependence of the preceding Volmer steps remains

$$\left.\frac{\partial \log_{10} j}{\partial \eta}\right|_{\log_{10}(1-\theta_{\mathrm{fcc}})=\mathrm{constant}} = \frac{2e+\beta_{\mathrm{T}}e}{2.303k_{\mathrm{B}}T} = \frac{2e}{2.303k_{\mathrm{B}}T}. \tag{67}$$

Now, we evaluate the potential dependence of the coverage term $(1-\theta_{\mathrm{fcc}})$

$$\frac{\partial \log_{10} j}{\partial \eta} = \frac{\partial \log_{10}(1-\theta_{\mathrm{fcc}})}{\partial \eta} + \frac{2e}{2.303k_{\mathrm{B}}T}, \tag{68}$$

where we use the expression for $1-\theta_{\mathrm{fcc}}$ from equation 64

$$\frac{\partial \log_{10} j}{\partial \eta} = \frac{\partial \log_{10}}{\partial \eta}\left(\frac{1}{1+\exp\left(-\frac{\Delta G^{\circ r}_{\mathrm{fcc}}-e\eta}{k_{\mathrm{B}}T}\right)}\right) + \frac{2e}{2.303k_{\mathrm{B}}T}. \tag{69}$$

The expression above can be simplified further

$$\log_{10}(1-\theta_{\mathrm{fcc}}) = \log_{10}\left(\frac{1}{1+\exp\left(-\frac{\Delta G^{\circ r}_{\mathrm{fcc}}-e\eta}{k_{\mathrm{B}}T}\right)}\right) = -\log_{10}\left(1+\exp\left(-\frac{\Delta G^{\circ r}_{\mathrm{fcc}}-e\eta}{k_{\mathrm{B}}T}\right)\right). \tag{70}$$

Here, we make use of the following logarithmic relation

$$\frac{d\log_{10} x}{dx} = \frac{d}{dx}\left(\frac{\ln x}{\ln 10}\right). \tag{71}$$

Thus, the partial derivative in equation 61 becomes

$$\frac{\partial \log_{10} j}{\partial \eta} = -\frac{1}{2.303}\frac{\partial}{\partial \eta}\left(\ln\left[1+\exp\left(-\frac{\Delta G^{\circ r}_{\mathrm{fcc}}-e\eta}{k_{\mathrm{B}}T}\right)\right]\right) + \frac{2e}{2.303k_{\mathrm{B}}T}, \tag{72}$$

and evaluation of the partial derivative yields

$$\frac{\partial \log_{10} j}{\partial \eta} = -\frac{e}{2.303 k_{\rm B} T} \left( \frac{\exp\left(-\frac{\Delta G^{\circ r}_{\rm fcc} - e\eta}{k_{\rm B}T}\right)}{1 + \exp\left(-\frac{\Delta G^{\circ r}_{\rm fcc} - e\eta}{k_{\rm B}T}\right)} \right) + \frac{2e}{2.303 k_{\rm B} T}. \tag{73}$$

If the reaction is strongly endergonic, the exponential term approaches zero. Conversely, if the reaction is highly exergonic, the exponential term is significantly larger than unity. This leads to the following relation

$$\frac{\partial \eta}{\partial \log_{10} j} = \begin{cases} \frac{2.303 k_{\rm B} T}{2e}, & \Delta G^{r}_{\rm fcc} >> 0 \\ \frac{2.303 k_{\rm B} T}{e}, & \Delta G^{r}_{\rm fcc} << 0 \\ \left[\frac{2.303 k_{\rm B} T}{2e}, \frac{2.303 k_{\rm B} T}{e}\right], & \text{otherwise} \end{cases}$$

At 298 K, these Tafel slopes correspond to

$$\frac{\partial \eta}{\partial \log_{10} j} = \begin{cases} 30 \text{ mV dec}^{-1}, & \Delta G^{r}_{\rm fcc} >> 0 \\ 60 \text{ mV dec}^{-1}, & \Delta G^{r}_{\rm fcc} << 0 \\ [30, 60] \text{ mV dec}^{-1}, & \text{otherwise} \end{cases}$$

We note that this analysis is also valid for rate-limiting Volmer, Heyrovsky and top-top Tafel mechanisms. However, the overpotential ($H_{\rm top}$) hydrogen coverage is always in the low limit at the potentials of interest for these mechanisms. Thus, the coverage is essentially independent of applied potential.

# 9 Linear response between reaction energy and applied potential

As noted in the main article, the reaction energy of the Volmer step changes linearly with applied potential. This is shown in Figure S8, where the reaction energies for ontop and fcc adsorption are plotted against the applied potential. The slopes are less than unity—a consequence of hybridization and fractional charge transfer.

# 10 Volmer reaction energetics as a function of unit cell size

The left panel of Figure S9 shows the unit cell size dependence of the reaction energetics of the Volmer reaction. We consider two unit cells: 3×2×3 and 3×3×3. These correspond to interfacial proton concentrations of $\frac{1}{4}$ and $\frac{1}{6}$, respectively. We see that the (potential) reaction energy and barrier only shift by ~60 meV when the proton concentration in the interface changes from $\frac{1}{4}$ to $\frac{1}{6}$. Moreover, the shape of the reaction barrier is independent of the unit cell size; that is, the reaction is essentially barrierless (Butler–Volmer symmetry

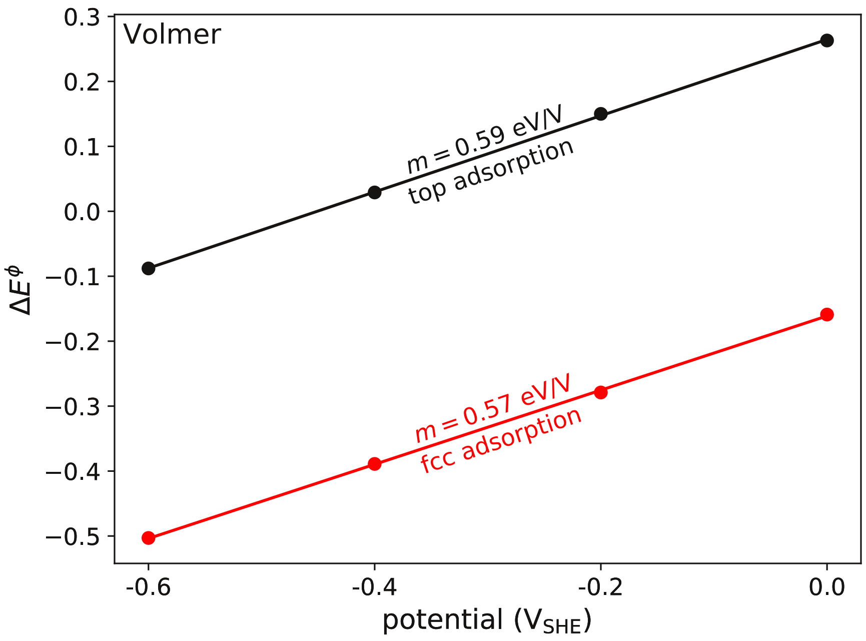


**Figure S8:** Reaction energies of the Volmer step as a function of applied potential. The reaction energy changes linearly with applied potential, and the slope is less than unity. The latter is a consequence of hybridization between the electrode and the solvated proton.

factor close to unity) in both unit cells. We interpret this small change in potential energy as a stabilization of the initial state when the proton concentration is decreased. However, the left panel shows the potential energy barrier; neither free energy corrections nor proton shuttling have been accounted for. At high proton concentrations in the interface, the pseudo-initial state is destabilized. However, the reduction in entropy is also more pronounced for the smaller unit cell. The right panel of Figure S9 shows the complete (*i.e.*, ∼1-electron transfer) for the two unit cells. Note that the reaction has a small forward reaction barrier in potential energy, but is barrierless in free energy for the 3×3×3 unit cell. Interestingly, the free energy difference between unit cell sizes is smaller than in potential energy. This is a consequence of partial cancellation of the potential energy and entropic differences.

# 11 Tafel reaction energetics as a function of water geometry

Figure S10 shows top–hollow Tafel barriers as a function of water geometry at the equilibrium potential. We consider three cases: (i) an adsorbed neutral water bilayer, (ii) an adsorbed acidic water bilayer, and (iii) without a water bilayer. The reaction exhibits a weak dependence on the water geometry; the reaction barrier changes by 0.06 eV between the extreme cases.

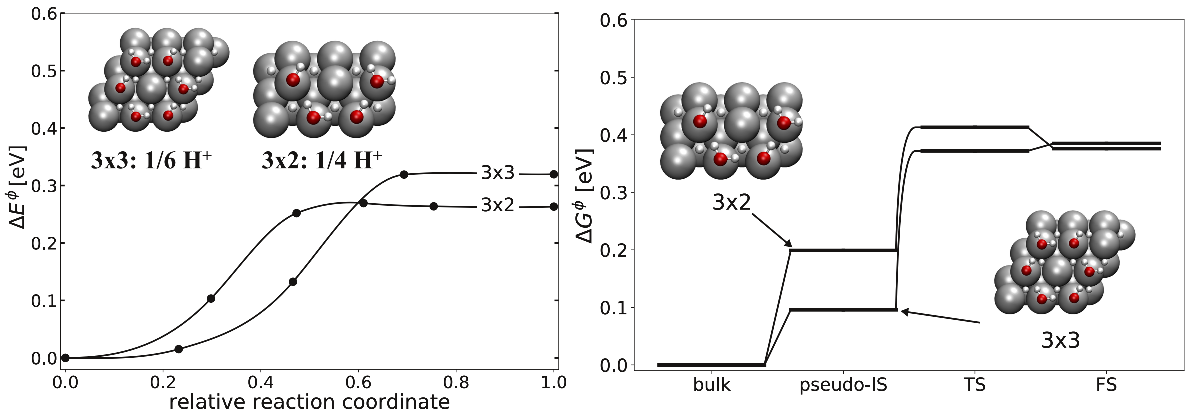


**Figure S9:** Left: Reaction energy and barrier of the Volmer step on Pt(111) as a function of unit cell size. Right: Free energy of the complete Volmer step (∼1-electron charge transfer) as a function of unit cell size.

# 12 Potential energy barriers on Au(111)

As noted in the main article, the Volmer reaction on Au(111) includes two distinct processes; an electrochemical reaction into an on-top site followed by exothermic diffusion into a neighboring fcc-hollow site. This is shown in the left panel of Figure S11, where the saddle point of the electrochemical step is marked with a circle. The reaction barrier is lower for the Heyrovsky reaction, shown in the right panel. We note that these are potential energy barriers. The free energy barriers of the Volmer and Heyrovsky steps at the equilibrium potential are 0.78 eV and 0.70 eV, respectively, when proton shuttling and free energy corrections are included.

# 13 Volmer reaction on Au(111) with different water geometries

*Ab initio* molecular dynamics studies suggest that hexagonal water structures are not stable on gold electrodes, and that the interfacial water is more disordered.[6] To study the effect of the interfacial water structure on the energetics of HER on Au, we have calculated the Volmer reaction with hexagonal water structures and cluster models, the latter of which has a Zundel ion ($H_5O_2^+$) as the proton donor. As shown in Figure S12, we find that the proton first deposits onto an ontop site regardless of interfacial water structure. The reaction pathway is independent of the initial location of the Zundel ion; if the cluster is located directly above an fcc site, the pathway includes a diffusion segment wherein the cluster moves towards an ontop site before depositing the proton. We interpret this is a consequence of distance; the energetic penalty associated with depositing a proton in an fcc site is higher than that of depositing the proton in an ontop site, since the distance between the proton and the ontop site is shorter.

Moreover, we find that the electron transfer profile is essentially identical between the

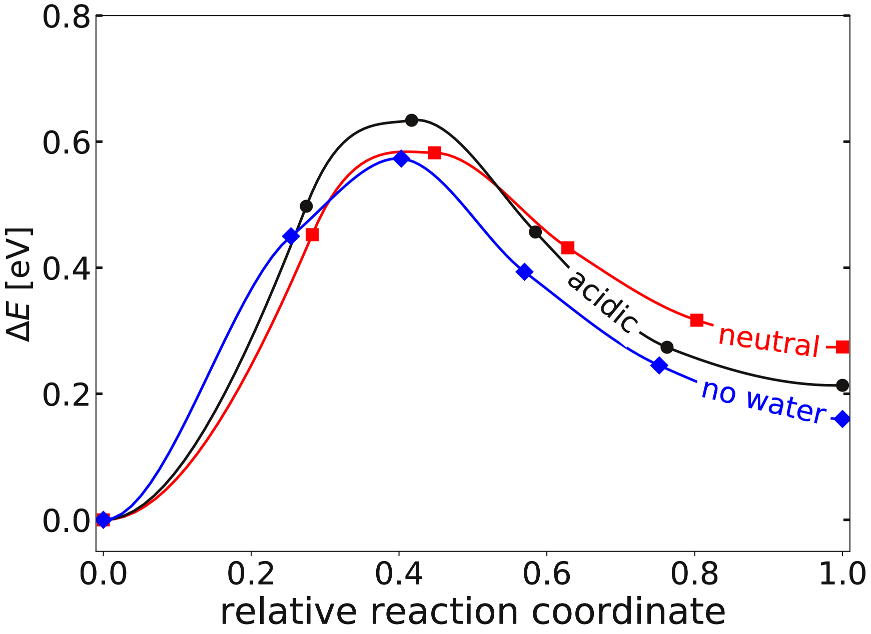


**Figure S10:** Tafel reaction barrier with a neutral water bilayer (red squares), with an acidic water bilayer (black circles) and without an adsorbed water bilayer (blue diamonds). The reaction barrier is essentially independent of the water geometry of the adsorbed bilayer.

two water structures; the electron transfer process ends at the ontop site, and the exothermic diffusion process between the two adsorption sites exhibits negligible potential dependence. This is shown for the Zundel ion in Figure S13 below, while the electron transfer profile for the hexagonal water structure is shown in Figure 5 of the main article.

# 14 Site-dependent Tafel reaction barriers

The reaction barrier of the Tafel reaction is highly dependent on the originating adsorption site. Figure S14 shows the Tafel barrier on Au(111) and Pt(111), where the hydrogens are adsorbed in top sites on Pt. The intrinsic reaction barrier of the top–top mechanism on Pt(111) is significantly lower than on Au(111); the barrier is $\sim 0.35$ eV less at the same thermodynamic driving force. The right panel of Figure S14 shows a BEP relation of selected fcc metals from ref. 4[7] as well as data from the current work. Although the data is sparse and somewhat scattered, we see that the top–top Tafel mechanism (labelled Pt(111)/tt) deviates from the scaling relation of the hollow-bound hydrogens.

# 15 Tafel barrier rationalization on the basis of a normal mode analysis

A qualitative picture for the relative barrier heights can be achieved from comparing the vibrational frequency of the normal mode representing the movement of the active hydrogens

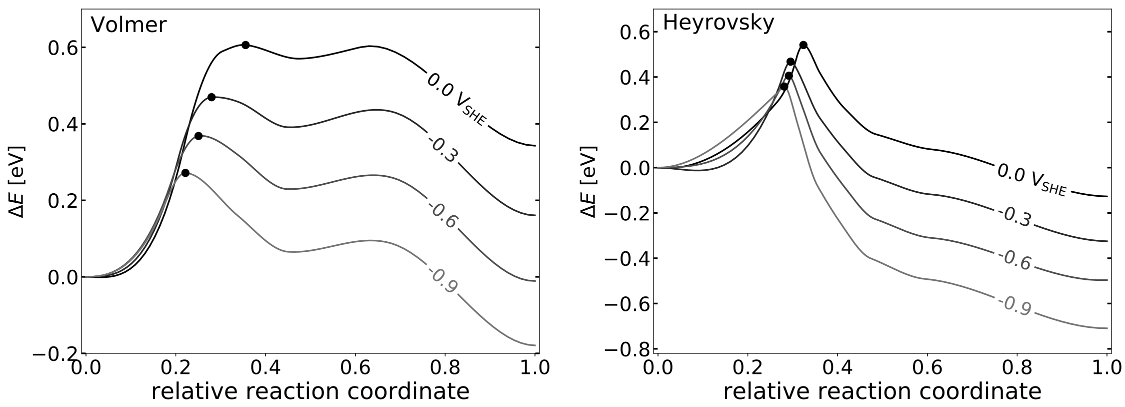


**Figure S11:** Potential energy reaction barriers for the Volmer and Heyrovsky steps on Au(111).

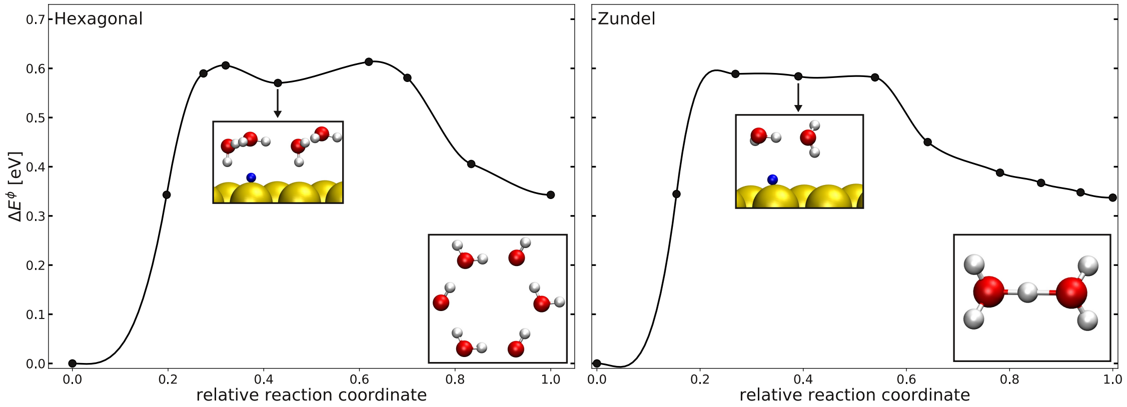


**Figure S12:** The Volmer reaction on Au(111) with different interfacial water structures. Regardless of the interfacial water structure, we find that the proton deposits in an ontop site before diffusing into an neighboring fcc site.

along the reaction coordinate. While the movement out of the initial state in the Tafel reaction involving hollow bound hydrogens on Au is dominated by the stretch vibration perpendicular to the electrode surface at $\sim 860$ cm$^{-1}$ (making up 73% of the movement), the top–top Tafel mechanism on Pt rather follows lateral modes at only $\sim 590$ cm$^{-1}$ (describing 81% of the movement), therefore facilitating the approach of the transition state.

# 16 Unit cell in SJ method

Figure S15 shows a typical unit cell within the SJ method. The unit cell includes an electrode, acidic (protonated) explicit water and implicit solvent. A Jellium counter charge (depicted by 45° lines) is immersed in the implicit solvent, and implicit solvent is only included on the reactive side of the electrode.

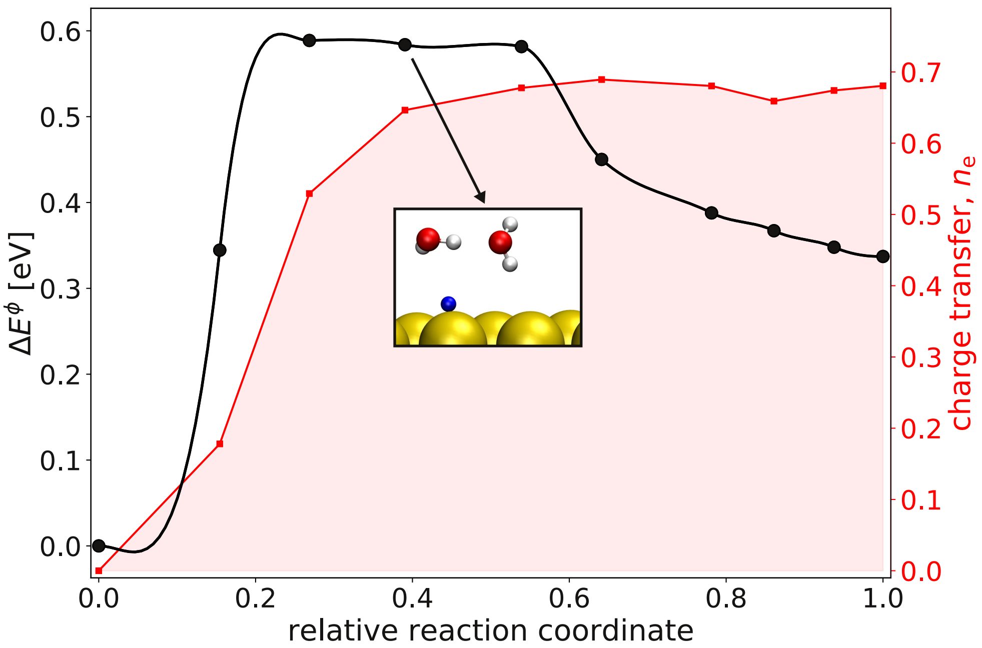


**Figure S13:** Reaction pathway and corresponding charge transfer for the Volmer reaction on Au(111) where the proton donor is a Zundel ($H_5O_2^+$) ion. The diffusion process between the two adsorption sites exhibits negligible potential dependence.

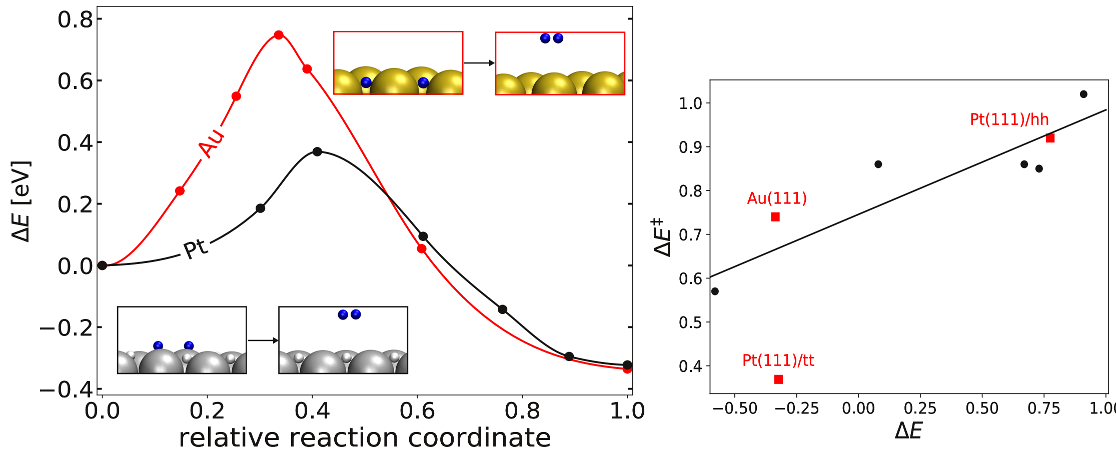


**Figure S14:** Left: Tafel barrier on Au(111) and Pt(111), where the reactive intermediates are adsorbed on-top of Pt. Right: BEP relation of the Tafel reaction on fcc metals (ref.[7]) as well as data from the current work (red points).

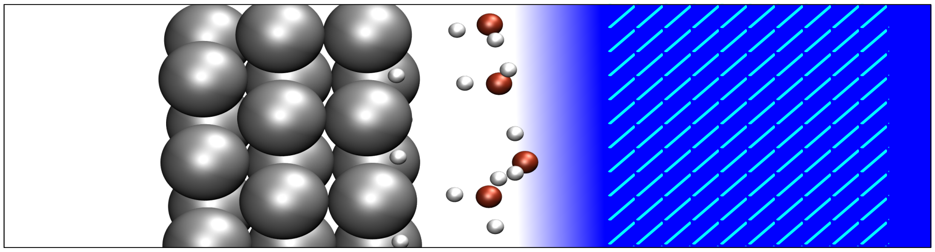

**Figure S15:** Unit cell in the $xz$-plane. The blue region and the 45° lines represent the implicit solvent and solvated counter charge, respectively.

# References


(1) Nørskov, J. K.; Rossmeisl, J.; Logadottir, A.; Lindqvist, L.; Kitchin, J. R.; Bligaard, T.; Jónsson, H. Origin of the Overpotential for Oxygen Reduction at a Fuel-Cell Cathode. *J. Phys. Chem. B* **2004**, *108*, 17886–17892.

(2) Trasatti, S. International Union of Pure and Applied Chemistry Commission on Electrochemistry * The Absolute Electrode Potential: An Explanatory note. *Pure Appl. Chem.* **1986**, *58*, 955–966.

(3) Kastlunger, G.; Lindgren, P.; Peterson, A. A. Controlled-potential simulation of elementary electrochemical reactions : proton discharge on metal surfaces. *J. Phys. Chem. C* **2018**, *122*, 12771–12781.

(4) Chen, L. D.; Bajdich, M.; Martirez, J. M. P.; Krauter, C. M.; Gauthier, J. A.; Carter, E. A.; Luntz, A. C.; Chan, K.; Nørskov, J. K. Understanding the apparent fractional charge of protons in the aqueous electrochemical double layer. *Nat. Commun.* **2018**, *9*, 3202.

(5) Henkelman, G.; Arnaldsson, A.; Jónsson, H. A fast and robust algorithm for Bader decomposition of charge density. *Comput. Mater. Sci.* **2006**, *36*, 354–360.

(6) Schnur, S.; Groß, A. Properties of metal–water interfaces studied from first principles. *New J. Phys.* **2009**, *11*, 125003.

(7) Wang, S.; Petzold, V.; Tripkovic, V.; Kleis, J.; Howalt, J. G.; Skúlason, E.; Fernández, E. M.; Hvolbæk, B.; Jones, G.; Toftelund, A.; Falsig, H.; Björketun, M.; Studt, F.; Abild-Pedersen, F.; Rossmeisl, J.; Nørskov, J. K.; Bligaard, T. Universal transition state scaling relations for (de)hydrogenation over transition metals. *Phys. Chem. Chem. Phys.* **2011**, *13*, 20760–20765.
